# Supplementary material for: Scale-Adaptive Feature Aggregation for Efficient Space-Time Video Super-Resolution
Source: arXiv:2310.17294 source file (2023-11-27)
Supplement: Supplementary file 1 [file appendix.tex]

\begin{figure}[tb]
	\centering
	\includegraphics[width=8cm]{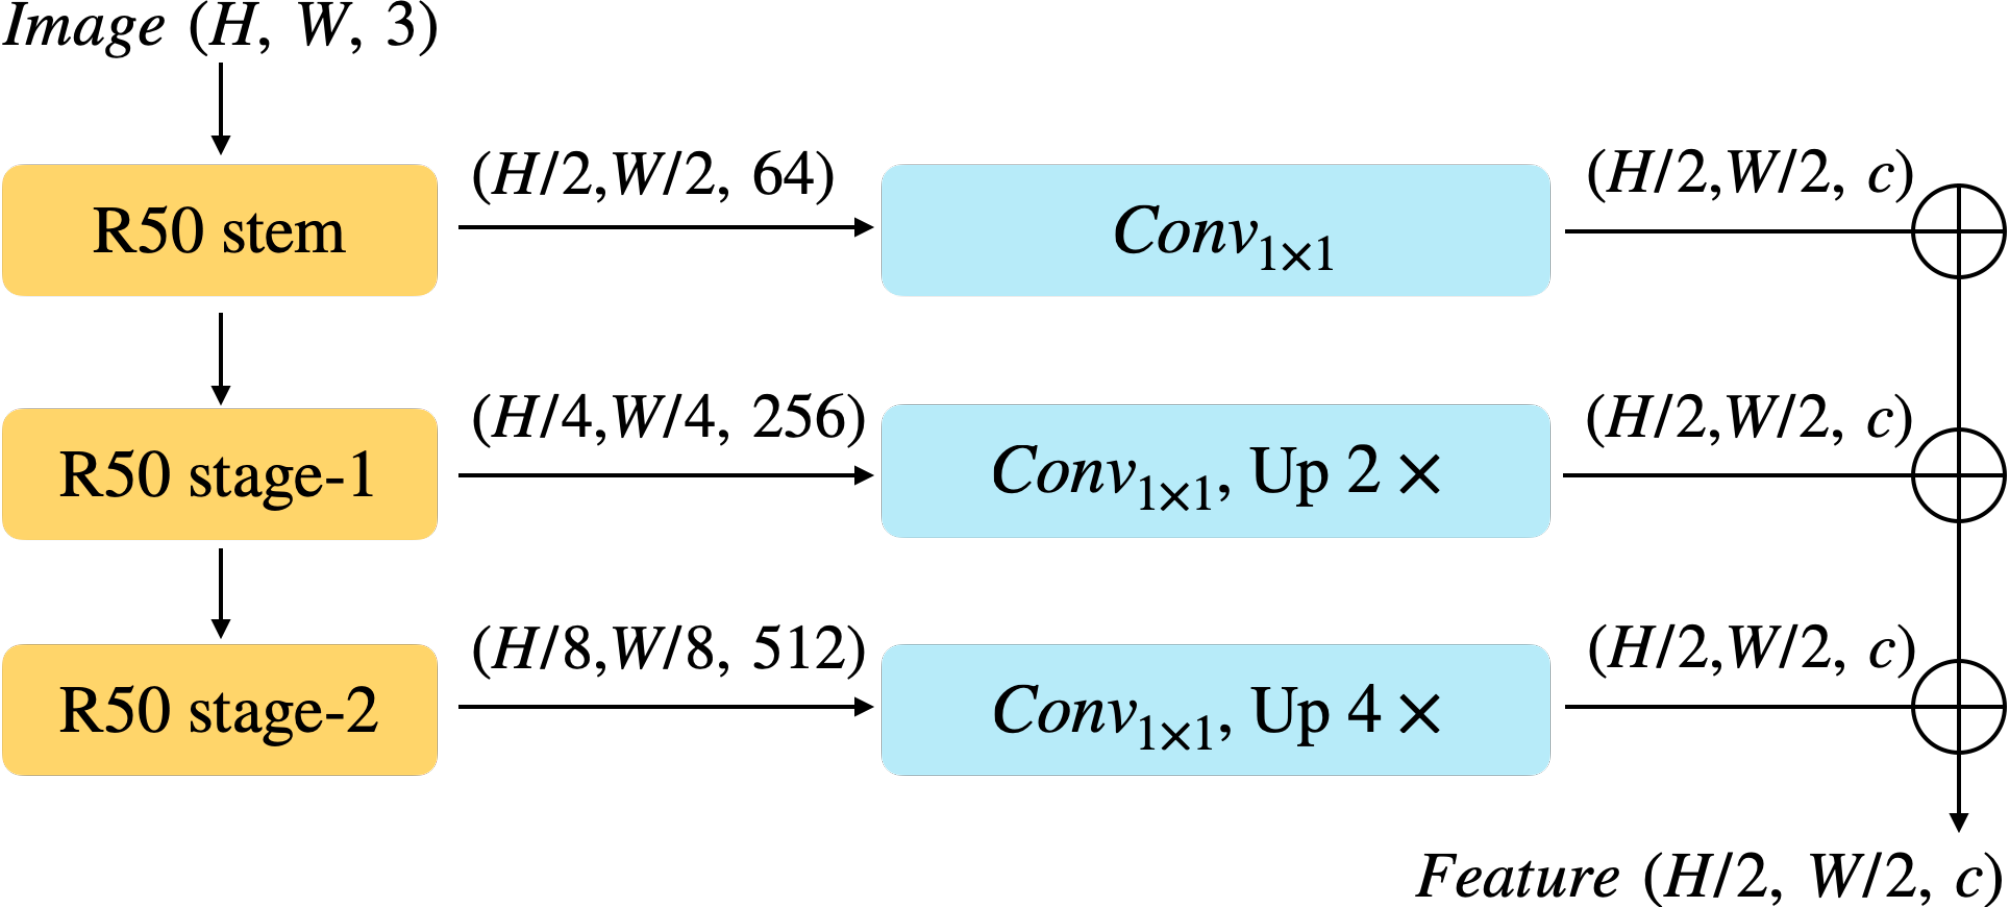}
	\caption{\textbf{Ours feature extractor $\mathcal{E}$ based on ResNet-50~(R50)~\cite{he2016deep}}} 
	\label{fig:head}
\end{figure}
